# Supplementary material for: Gate-Control of Spin Precession in Quantum Hall Edge States
Source: arXiv:1207.7243 source file (2012-08-02)
Supplement: Supplementary file 1 [file SubmittedSupplement_July27.pdf]

# Supplemental Material for "Gate-Control of Spin Precession in Quantum Hall Edge States"

T. Nakajima,[1,*] Kuan-Ting Lin,[2] and S. Komiyama[1]

[1]*Department of Basic Science, University of Tokyo, Komaba, Meguro-ku, Tokyo 153-8902, Japan*

[2]*Department of Physics, National Tsing Hua University, Hsinchu 30013, Taiwan*

## Abstract

Additional details including device structures and influence of random potentials are discussed.

## I. HETEROSTRUCTURES AND DEVICES

Two sets of experimental devices (Figs. 1(a), (b) and the left panel of Fig. 2(a)) and control devices (the right panel of Fig. 2(a) and Fig. S1 below) were fabricated, respectively, in two different modulation-doped GaAs/AlGaAs heterostructure crystals, I and II. Heterostructure of crystal I consists of a $1\,\mu$m GaAs layer, a 20 nm AlGaAs barrier layer, a 60 nm Si-doped AlGaAs layer, and a 10 nm GaAs cap layer. That of crystal II consists of a $1\,\mu$m GaAs layer, a 40 nm AlGaAs barrier layer, a Si $\delta$-doping layer, a 60 nm AlGaAs layer, and a 10 nm GaAs cap layer. The 2D electron densities $n$ and the electron mobilities $\mu$ at 4.2 K are $n = 2.4 \times 10^{15}\,\mathrm{m}^{-2}$ and $\mu = 67\,\mathrm{m}^2/\mathrm{Vs}$ in crystal I and $n = 2.0 \times 10^{15}\,\mathrm{m}^{-2}$ and $\mu = 71\,\mathrm{m}^2/\mathrm{Vs}$ in crystal II. Ohmic contacts were prepared by alloying 200 nm-thick AuGe/Ni after mesa structures were defined by wet etching. Cross gates (only in the experimental devices) and side gates were patterned by electron-beam lithography followed by deposition of a 80 nm-thick Ti layer and the lift-off process.

The device structure for control experiments (the right panel of Fig. 2(a)) is shown in Fig. S1. After the process of mesa etching, ohmic contact alloying and side gate (SG) deposition, the entire device surface was covered with a 100 nm-thick aluminum oxide layer for insulation. Cross gates (CGs) were patterned by depositing a 30 nm-thick Ti layer and a 120 nm-thick Au layer on top of the insulating layer, forming finite overlap with side-gate regions. In this geometry, SG corners are absent along the up-spin edge-state trajectory (red line). Furthermore, the bend of the down-spin edge-state trajectory (blue line) is made substantially smoother due to increased distance to the CGs. Inter-edge state scattering at the entrance of the SG is thereby completely suppressed.

## II. OSCILLATIONS IN $T_{\uparrow\uparrow}$

Several additional data of $T_{\uparrow\uparrow}$ demonstrating oscillations against $B$ and $V_{\mathrm{SG}}$ are displayed, respectively, in Figs. S2(a) and S2(c) for $L = 5\,\mu$m and $10\,\mu$m regions. Fourier spectra of respective oscillations are shown in Figs. S2(b) and S2(d).

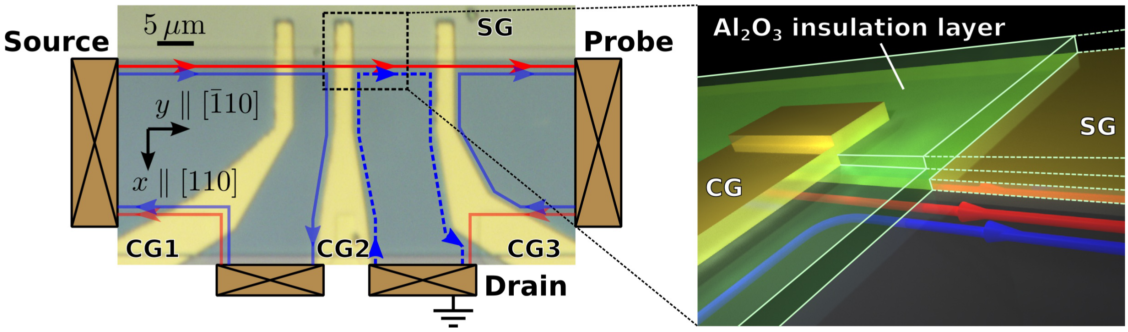


Figure S1. Optical microscope image of the device for the control experiments (left) and an enlarged schematic view illustrating the structure in the vicinity of the "entrance" to SG region (right).

## III. INFLUENCE OF RANDOM POTENTIALS

In general, locally varying electric fields can cause elastic inter-edge state scattering via SOI[1,2]. It should be noted, however, that the experimental results discussed in the present work are free from the effects of individual impurities or defects located in the close vicinity of edge states. It is experimentally established that those individual scatterers are addressable as finger-print-like irregular structures when the Hall voltage is studied while the 2D electron system is scanned with edge states[3–5]. The oscillatory structure discussed in the present work is distinctly different from those irregular structures.

To show this unambiguously, we display in the upper panel of Fig. S3 an example of $T_{\uparrow\uparrow}$ vs $V_{\mathrm{SG}}$ curve at $B = 3.65\,\mathrm{T}$ which is featured by impurity-induced irregular structures. Three distinct sharp dips (maked by arrows) correspond to respective scatterers: The scattering probability sharply increases ($T_{\uparrow\uparrow}$ drops) when the edge states crosses the site of particular scatterers as $V_{\mathrm{SG}}$ is changed. These impurity-induced structures are irregular and can be distinguished from regular oscillatory structures, as is readily confirmed in the Fourier analysis. Moreover, the individual scatterers give rise to clear "scars" in the 2D plot of $T_{\uparrow\uparrow}$ on the plane of $B$ and $V_{\mathrm{SG}}$ as shown in the lower panel of Fig. S3, which are easily distinguished from the oscillatory pattern discussed in this work. The "scars" are nearly vertical in the lower panel of Fig. S3 because the locations of scatterers and edge states are almost independent of $B$ (see Fig. 4(b)).

Statistical fluctuation in the remote impurity distribution is known to introduce slowly varying random potential in modulation-doped heterostructures and significantly influence the property of high-mobility 2D electron systems. The resulting long-range random po-

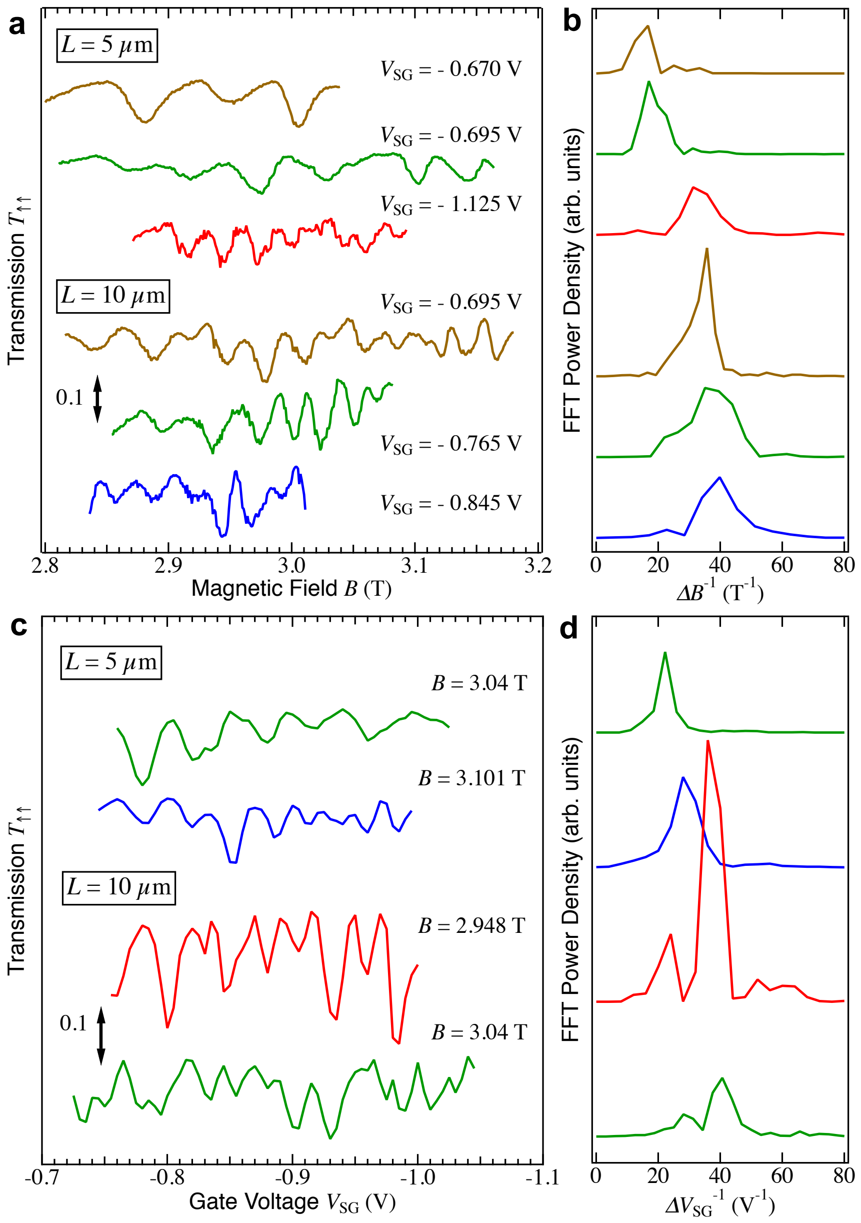


Figure S2. Curves of $T_{\uparrow\uparrow}$ exemplifying the oscillations representing spin precession. Curves of $T_{\uparrow\uparrow}$ vs $B$ at fixed $V_{\rm SG}$ are shown in (a) with corresponding Fourier spectra in (b). Curves of $T_{\uparrow\uparrow}$ vs $V_{\rm SG}$ at fixed $B$ are shown in (c) with corresponding Fourier spectra in (d).

tential ($\gg \ell_{\rm B}$) does not effectively cause spin-split inter-edge state scattering but leads to irregular trajectory of edge states in the slowly varying potential landscape[6,7]. Since the detailed profile of edge-state trajectories fluctuates with varying $B$ and $V_{\rm SG}$, the effective length of edge states $L$, the edge-state separation $\Delta x$, and the group velocity $\boldsymbol{v}_g$ fluctuate accordingly with $B$ and $V_{\rm SG}$. This is supposed to be the mechanism of the experimentally

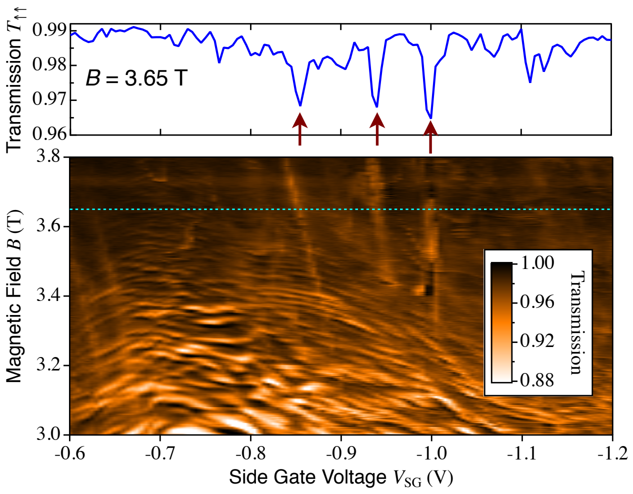


Figure S3. $T_{\uparrow\uparrow}$ obtained in the region of $L = 5\,\mu$magainst $V_{SG}$ at $B = 3.65\,$T (lower panel). The lower panel is a 2D plot on the plane of $B$ and $V_{SG}$.

observed irregular distortion in the oscillatory pattern of $T_{\uparrow\uparrow}$ (Figs. 3(a) and S3). (The scattering matrices $S_L$ and $S_R$ may be influenced by $B$ and $V_{SG}$ as well, but this effect will lead to only small deviation of $C_0$, $C_1$, and $\phi_0$ in eq. 2.)

## IV. SMALL DC-BACKGROUND VOLTAGE IN SOURCE-DRAIN BIAS

In the present experiments a constant negative dc voltage is applied for the source-drain bias ($V_S = V_{dc} + V_{ac}$ with $V_{dc} = -103\,\mu$V ). This is for obtaining excellent visibility in oscillation of $T_{\uparrow\uparrow}$ as described below.

When a positive bias voltage is applied, spin-flip inter-edge state scattering (taking place along the SG boundary) increases dramatically as shown in Fig. S4: Complete equilibration of edge states ($T_{\uparrow\uparrow} \approx 0.5$) is achieved already at $V_{dc} \approx 100\,\mu$V. For $V_{dc} > 0$, the outer up-spin edge state has a lower electrochemical potential, and strong inter-edge state scattering is supposed to be introduced as schematically shown in the right inset of Fig. S4[8,9]. The inter-edge state scattering rate is substantially lower at $V_{dc} = 0$ and, interestingly, the scattering is suppressed further for $V_{dc} < 0$. As shown in Fig. S4, $T_{\uparrow\uparrow}$ exceeds 0.9 with small negative bias voltages ($-40 < V_{dc} < -180\,\mu$V) and the experimentally applied voltage ($V_{dc} = -103\,\mu$V) is marked by an arrow. The lower scattering rate may be ascribed to the fact that the scattering is possible only via tunneling through the barrier of an incompressible region as shown in

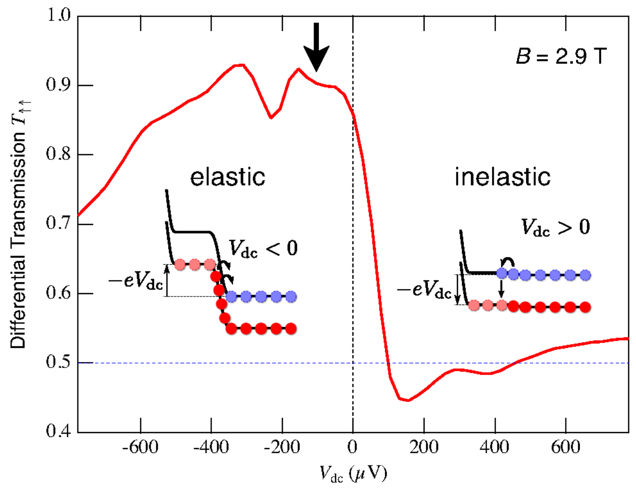


Figure S4. Differential transmission probability $T_{\uparrow\uparrow}$ ($L = 5\,\mu$m) as a function of $V_{dc}$ ($V_{ac} = 12.9\,\mu$V) taken at $B = 2.9$ T. The insets show the edge-state energy level diagram for respective polarities of $V_{dc}$.

the left inset of Fig. S4 when the outer (up-spin) edge state has a higher electrochemical potential for $V_{dc} < 0$. It follows that a small negative bias is helpful for better visibility of oscillation in $T_{\uparrow\uparrow}$.

With a finite dc source-drain voltage, nuclear spins are dynamically polarized[4,8,10]. In the present experiments, this effect is canceled out by applying a counter (positive) dc voltage after each run of measurements.

---


* nakajima@meso.t.u-tokyo.ac.jp



1 A. V. Khaetskii, Phys. Rev. B **45**, 13777 (1992).

2 D. G. Polyakov, Phys. Rev. B **53**, 15777 (1996).

3 Y. Acremann, T. Heinzel, K. Ensslin, E. Gini, H. Melchior, and M. Holland, Phys. Rev. B **59**, 2116 (1999).

4 T. Nakajima, Y. Kobayashi, S. Komiyama, M. Tsuboi, and T. Machida, Phys. Rev. B **81**, 085322 (2010).

5 N. Paradiso, S. Heun, S. Roddaro, D. Venturelli, F. Taddei, V. Giovannetti, R. Fazio, G. Biasiol, L. Sorba, and F. Beltram, Phys. Rev. B **83**, 155305 (2011).

6 T. Machida, S. Ishizuka, S. Komiyama, K. Muraki, and Y. Hirayama, Phys. Rev. B **63**, 045318

(2001).

[7] S. Ilani, J. Martin, E. Teitelbaum, J. H. Smet, D. Mahalu, V. Umansky, and A. Yacoby, Nature **427**, 328 (2004).

[8] D. C. Dixon, K. R. Wald, P. L. McEuen, and M. R. Melloch, Phys. Rev. B **56**, 4743 (1997).

[9] A. Würtz, R. Wildfeuer, A. Lorke, E. V. Deviatov, and V. T. Dolgopolov, Phys. Rev. B **65**, 075303 (2002).

[10] K. R. Wald, L. P. Kouwenhoven, P. L. McEuen, N. C. van der Vaart, and C. T. Foxon, Phys. Rev. Lett. **73**, 1011 (1994).
